# Supplementary material for: Privacy-Preserving News Recommendation Model Learning
Source: arXiv:2003.09592 source file (2020-10-08)
Supplement: Supplementary file 1 [file Supplement.tex]

\section*{Supplement}

\subsection*{Experiment Environment}

In this section, we introduce the environment of our experiments.
We conduct experiments on a server with Ubuntu 16.04.6 operating system.
There are 6 CPUs (Intel Xeon E5-2690 v4) and one GPU (Nvidia Tesla P100) in this server.
These approaches are implemented based on python (3.6).
The neural approaches are based on Keras\footnote{https://github.com/keras-team/} (2.2.4) deep learning framework with tensorflow\footnote{https://www.tensorflow.org/} (1.13.0) as backend.

\subsection*{Dataset Construction}
We collect user logs from a commercial news website between October 19 and November 15 to construct the dataset.
We randomly sample 100k users who had at least three clicked news in the five weeks.
To simulate the real scenario that not all of the users can be involved in the training stage, we randomly sample 50k users for model training and use 100k users for evaluation.

\subsection*{Data Preprocessing}
For fair comparisons, all methods are trained and evaluated based on the same processed data.
The news titles are converted to word sequences and we only retain the first 30 words.
We use the recent 50 clicked news before the impression time for user representation learning.

\subsection*{Hyperparameter Settings}
The hyper-parameters used in our approach are summarized in Table~\ref{hyper}.

\begin{table}[h]
\centering
\resizebox{0.8\linewidth}{!}{
\begin{tabular}{|l|c|}
\hline
\multicolumn{1}{|c|}{\textbf{Hyperparameters}}& \textbf{Value} \\ \hline
word embedding dimension                     & 300            \\
GRU units                                   &   400 \\
\# heads of multi-head attention networks                 & 20             \\
output dim of attention head               & 20            \\
dim of attention query             & 200            \\
strength of noise $\lambda$        & 0.015      \\
clipping value $\delta$                   & 0.005   \\
dropout ratio                       & 0.2            \\
optimizer                                    & SGD           \\
learning rate                                & 0.5           \\
batch size                                   & 32    \\     
training epoch                                   & 2    \\  

\hline
\end{tabular}
}
\caption{Detailed settings of hyperparameters.}\label{hyper}
\end{table}

\subsection*{Model Computational Cost}

There are 2.6 M parameters in the \textit{FedNewsRec} model except for the word embedding layer.
There are 19.5 M parameters in the word embedding layer.
It takes 813 seconds to train \textit{FedNewsRec} for one epoch.
